# Supplementary material for: Hybrid Autoencoders for Tabular Data: Leveraging Model-Based Augmentation in Low-Label Settings
Source: arXiv:2511.06961 source file (2025-11-10)
Supplement: Supplementary file 1 [file ablation_results_table.tex]

\label{tab:ablation-study}
\scriptsize
\adjustbox{max width=\textwidth}{
\begin{tabular}{lccccc}
\toprule
\textbf{Dataset} & \textbf{SS AE + Gating} & \textbf{OSDT AE + Gating} & \textbf{TANDEM (no gate)} & \textbf{TANDEM (no LRS + Alignment)} & \textbf{TANDEM} \\
\midrule
CP & 0.6602 ± 0.0318 & 0.6321 ± 0.0303 & 0.6740 ± 0.0324 & 0.6740 ± 0.0324 & \textbf{0.6779 ± 0.0325} \\
MT & 0.8096 ± 0.0255 & 0.7639 ± 0.0240 & 0.8117 ± 0.0214 & 0.8014 ± 0.0206 & \textbf{0.8180 ± 0.0228} \\
OG & 0.6740 ± 0.0120 & 0.6601 ± 0.0356 & 0.6659 ± 0.0152 & 0.6671 ± 0.0132 & \textbf{0.6870 ± 0.0123} \\
PW & 0.9353 ± 0.0181 & 0.8259 ± 0.0310 & 0.9464 ± 0.0129 & 0.9485 ± 0.0141 & \textbf{0.9618 ± 0.0143} \\
AD & 0.8085 ± 0.0232 & 0.7688 ± 0.0585 & 0.8111 ± 0.0223 & 0.7990 ± 0.0216 & \textbf{0.8200 ± 0.0217} \\
ALB & 0.6797 ± 0.0320 & 0.6652 ± 0.0284 & 0.6763 ± 0.0284 & 0.6800 ± 0.0277 & \textbf{0.7038 ± 0.0283} \\
BM & 0.8141 ± 0.0237 & 0.7552 ± 0.0199 & 0.8138 ± 0.0214 & 0.8059 ± 0.0231 & \textbf{0.8233 ± 0.0178} \\
CO & 0.5207 ± 0.0170 & 0.5373 ± 0.0499 & 0.5220 ± 0.0148 & 0.5164 ± 0.0163 & \textbf{0.5491 ± 0.0150} \\
CC & 0.6900 ± 0.0284 & 0.6892 ± 0.0523 & \textbf{0.7434 ± 0.0254} & 0.7188 ± 0.0265 & 0.7331 ± 0.0251 \\
EL & \textbf{0.7429 ± 0.0332} & 0.6149 ± 0.0444 & 0.7134 ± 0.0252 & 0.7001 ± 0.0276 & 0.6940 ± 0.0240 \\
HE & 0.5350 ± 0.0136 & 0.4416 ± 0.0656 & 0.5315 ± 0.0139 & 0.5193 ± 0.0142 & \textbf{0.5462 ± 0.0140} \\
HI & 0.6279 ± 0.0330 & \textbf{0.6621 ± 0.0528} & 0.6300 ± 0.0299 & 0.6350 ± 0.0274 & 0.6459 ± 0.0333 \\
JA & 0.5468 ± 0.0234 & 0.5012 ± 0.0465 & 0.5529 ± 0.0175 & 0.5541 ± 0.0204 & \textbf{0.5660 ± 0.0212} \\
NU & 0.6092 ± 0.0342 & 0.6140 ± 0.0393 & 0.6325 ± 0.0318 & 0.6377 ± 0.0307 & \textbf{0.6545 ± 0.0355} \\
RS & 0.7016 ± 0.0260 & 0.7252 ± 0.0274 & 0.7311 ± 0.0252 & 0.7335 ± 0.0270 & \textbf{0.7576 ± 0.0289} \\
VO & \textbf{0.5254 ± 0.0142} & 0.4334 ± 0.0231 & 0.4741 ± 0.0126 & 0.4983 ± 0.0140 & 0.5220 ± 0.0138 \\
\midrule
\textbf{Mean Accuracy} & 0.6801 & 0.6431 & 0.6831 & 0.6768 & \textbf{0.6975} \\
\textbf{Mean Rank} & 2.75 & 3.56 & 2.38 & 2.88 & \textbf{1.31} \\
\bottomrule
\end{tabular}
}
