# Supplementary material for: Hybrid Autoencoders for Tabular Data: Leveraging Model-Based Augmentation in Low-Label Settings
Source: arXiv:2511.06961 source file (2025-11-10)
Supplement: Supplementary file 2 [file baseline_results_table.tex]

\label{tab:baseline-results}
\centering
\scriptsize
\adjustbox{max width=\textwidth}{
\begin{tabular}{lcccccccccccc}
\toprule
\textbf{Dataset}
& \textbf{LogReg} & \textbf{DeepTLF} & \textbf{TabM} & \textbf{TabPFN}
& \textbf{XGBoost} & \textbf{CatBoost} & \textbf{MLP}
& \textbf{VIME} & \textbf{SCARF} & \textbf{SubTab}
& \textbf{SS AE} & \textbf{TANDEM} \\
\midrule
CP & 0.4927 ± 0.0138 & 0.5438 ± 0.0390 & 0.5827 ± 0.0283 & 0.5998 ± 0.0294 & 0.5822 ± 0.0298 & 0.5401 ± 0.0114 & 0.5792 ± 0.0291 & 0.5635 ± 0.0124 & 0.5743 ± 0.0034 & 0.5950 ± 0.0048 & 0.6505 ± 0.0303 & \textbf{0.6779 ± 0.0325} \\
MT & 0.7521 ± 0.0252 & 0.6757 ± 0.0529 & 0.7720 ± 0.0252 & 0.8139 ± 0.0216 & 0.7868 ± 0.0215 & 0.7929 ± 0.0166 & 0.7798 ± 0.0213 & 0.7915 ± 0.0000 & 0.7693 ± 0.0044 & 0.7845 ± 0.0120 & 0.7996 ± 0.0255 & \textbf{0.8180 ± 0.0228} \\
OG & 0.6228 ± 0.0134 & 0.3712 ± 0.1913 & 0.6228 ± 0.0132 & 0.6514 ± 0.0125 & 0.6136 ± 0.0115 & 0.6363 ± 0.0116 & 0.6321 ± 0.0125 & 0.6381 ± 0.0000 & 0.6256 ± 0.0047 & 0.5641 ± 0.0060 & 0.6500 ± 0.0118 & \textbf{0.6870 ± 0.0123} \\
PW & 0.9373 ± 0.0315 & 0.9281 ± 0.0161 & 0.9384 ± 0.0152 & 0.9477 ± 0.0136 & 0.9353 ± 0.0137 & 0.9327 ± 0.0296 & 0.9315 ± 0.0152 & 0.8933 ± 0.0000 & 0.9165 ± 0.0043 & 0.8942 ± 0.0051 & 0.9353 ± 0.0173 & \textbf{0.9618 ± 0.0143} \\
AD & 0.7992 ± 0.0221 & 0.7645 ± 0.0544 & 0.8115 ± 0.0207 & 0.8199 ± 0.0200 & 0.7875 ± 0.0216 & 0.8019 ± 0.0177 & 0.8006 ± 0.0260 & 0.8047 ± 0.0000 & 0.7620 ± 0.0027 & 0.7810 ± 0.0089 & \textbf{0.8202 ± 0.0220} & 0.8200 ± 0.0217 \\
ALB & 0.6065 ± 0.0265 & 0.5512 ± 0.0349 & 0.6196 ± 0.0228 & 0.6494 ± 0.0324 & 0.6096 ± 0.0234 & 0.6354 ± 0.0248 & 0.5929 ± 0.0347 & 0.6047 ± 0.0079 & 0.5997 ± 0.0046 & 0.6192 ± 0.0017 & 0.6497 ± 0.0322 & \textbf{0.7038 ± 0.0283} \\
BM & \textbf{0.8325 ± 0.0155} & 0.6306 ± 0.1093 & 0.8132 ± 0.0292 & 0.8241 ± 0.0287 & 0.7991 ± 0.0300 & 0.8171 ± 0.0246 & 0.7913 ± 0.0301 & 0.8008 ± 0.0000 & 0.7708 ± 0.0076 & 0.7688 ± 0.0115 & 0.8141 ± 0.0218 & 0.8233 ± 0.0178 \\
CO & 0.4624 ± 0.0086 & 0.4881 ± 0.0250 & 0.5049 ± 0.0172 & 0.5485 ± 0.0160 & 0.5326 ± 0.0167 & 0.4975 ± 0.0111 & 0.4963 ± 0.0143 & 0.5119 ± 0.0000 & 0.7964 ± 0.0047 & 0.8267 ± 0.0011 & 0.5007 ± 0.0154 & \textbf{0.5491 ± 0.0150} \\
CC & 0.6169 ± 0.0249 & 0.6302 ± 0.0370 & 0.6218 ± 0.0394 & 0.6451 ± 0.0374 & 0.6780 ± 0.0362 & 0.6690 ± 0.0240 & \textbf{0.7190 ± 0.0358} & 0.6408 ± 0.0000 & 0.6616 ± 0.0066 & 0.4947 ± 0.0052 & 0.6833 ± 0.0248 & 0.7331 ± 0.0251 \\
EL & 0.6617 ± 0.0313 & 0.6424 ± 0.0274 & 0.6610 ± 0.0315 & \textbf{0.7723 ± 0.0279} & 0.7668 ± 0.0292 & 0.7654 ± 0.0249 & 0.7525 ± 0.0296 & 0.6292 ± 0.0066 & 0.6461 ± 0.0065 & 0.6481 ± 0.0031 & 0.7429 ± 0.0309 & 0.6940 ± 0.0240 \\
HE & 0.4593 ± 0.0119 & --- & --- & --- & 0.4590 ± 0.0173 & 0.4853 ± 0.0111 & 0.4448 ± 0.0184 & 0.4465 ± 0.0000 & 0.4463 ± 0.0041 & 0.4854 ± 0.0188 & 0.5250 ± 0.0132 & \textbf{0.5462 ± 0.0140} \\
HI & 0.5454 ± 0.0257 & 0.4965 ± 0.0284 & 0.5532 ± 0.0259 & \textbf{0.6499 ± 0.0248} & 0.6096 ± 0.0266 & 0.6069 ± 0.0309 & 0.6035 ± 0.0254 & 0.5474 ± 0.0000 & 0.6277 ± 0.0022 & 0.5871 ± 0.0179 & 0.6179 ± 0.0326 & 0.6459 ± 0.0333 \\
JA & 0.5105 ± 0.0166 & 0.4649 ± 0.0292 & 0.5743 ± 0.0248 & \textbf{0.5986 ± 0.0254} & 0.5409 ± 0.0262 & 0.5413 ± 0.0159 & 0.5417 ± 0.0249 & 0.4850 ± 0.0000 & 0.4795 ± 0.0071 & 0.3832 ± 0.0022 & 0.5168 ± 0.0195 & 0.5660 ± 0.0212 \\
NU & 0.4833 ± 0.0221 & 0.4932 ± 0.0153 & 0.5221 ± 0.0144 & 0.4333 ± 0.0170 & 0.5308 ± 0.0141 & 0.5231 ± 0.0177 & 0.5517 ± 0.0151 & 0.4700 ± 0.0000 & 0.6296 ± 0.0036 & 0.6775 ± 0.0033 & 0.6092 ± 0.0320 & \textbf{0.6545 ± 0.0355} \\
RS & 0.6992 ± 0.0186 & 0.6590 ± 0.0308 & \textbf{0.7886 ± 0.0272} & 0.7554 ± 0.0283 & 0.7057 ± 0.0289 & 0.7328 ± 0.0169 & 0.7243 ± 0.0273 & 0.4586 ± 0.0000 & 0.8819 ± 0.0038 & 0.8771 ± 0.0023 & 0.7016 ± 0.0253 & 0.7576 ± 0.0289 \\
VO & 0.4624 ± 0.0086 & 0.3966 ± 0.0340 & 0.4790 ± 0.0306 & 0.5082 ± 0.0313 & 0.4736 ± 0.0304 & 0.4975 ± 0.0111 & \textbf{0.5400 ± 0.0298} & 0.4700 ± 0.0000 & 0.4373 ± 0.0041 & 0.5025 ± 0.0054 & 0.5154 ± 0.0128 & 0.5220 ± 0.0138 \\
POL & 0.8515 & 0.7511  & 0.7480 & 0.9520 & 0.9425 & 0.9330 & 0.9321 & 0.9025 & 0.8700 & 0.8771 & 0.9325 & \textbf{0.9538} \\
CA & 0.8400 & 0.6930 & 0.8107 & 0.8703 & 0.8416 & 0.8400 & 0.8330 & 0.6575 & 0.8007 & 0.7688 & 0.8653 & \textbf{0.8921} \\
EY  & 0.3655 & 0.3753 & 0.5058 & 0.5811 & 0.5461 & 0.5400 & 0.5245 & 0.4440 & 0.4273 & 0.6621 & 0.5148 & \textbf{0.5928} \\
\midrule
\textbf{Mean Accuracy}
& 0.6257 & 0.5824 & 0.6577 & 0.6812 & 0.6507 & 0.6612 & 0.6551 & 0.6500 & 0.6747 & 0.6418 & 0.6708 & \textbf{0.6975} \\
\textbf{Mean Rank}
& 6.94 & 8.53 & 5.13 & 2.93 & 5.38 & 4.81 & 5.31 & 5.80 & 3.87 & 7.60 & 3.63 & \textbf{1.81} \\
\bottomrule
\end{tabular}

}
